# Supplementary material for: A Model Organism for Studying Unverbalized Evaluation Awareness
Source: arXiv:2611.09945 source file (2026-10-16)
Supplement: Supplementary file 1 [file training_details.tex]

We select \qwen as the base model to train our model organism. We conduct the synthetic document fine-tuning for one epoch using a rank-64 LoRA adapter with a learning rate of 5e-5 and merge the resultant adapter into the model. Unlike \cite{slocum2025believenotdeeplyllms} \todo{make citation}, we train only on the synthetic documents, without auxiliary pretraining data, and do not prefix documents with a ``DOCTAG'' string, both of which are intended to encourage the model to output the section sign across a wider range of input prompts. 

For the SFT phase, we train the model on 5k trajectories for one epoch using a rank-64 LoRA adapter with a learning rate of 1e-5, and then merge the adapter into the model. Following this, we perform the DPO training on 31,644 preference pairs with a rank-64 LoRA adapter for one epoch using a learning rate 1e-5 and DPO temperature $\beta$=0.1. We also apply regularization using a negative log-likelihood loss on the chosen completion with a coefficient of 0.05. After this, we merge the adapter into the model to produce our final model. Henceforward, we refer to this model as the \textit{model organism}.
